# Supplementary material for: Symbolic Learning for Material Discovery
Source: arXiv:2312.11487 source file (2023-11-30)
Supplement: Supplementary file 1 [file C_generative_models.tex]

\section{Future work}\label{sec:app:generative_models}
\textbf{Integration with generative AI} Generative AI technologies such as transformer-based foundation models \cite{bommasani2021opportunities}, and Generative Flow Networks (GFlowNets) \cite{bengio2021flow} are being used to propose new material candidates \cite{anstine2023generative, gupta2022matscibert, D3DD00002H, takeda2023foundation, yang2021transformer}. Foundation models however, are known to hallucinate, and GFlowNets rely on a human engineered and computationally efficient reward function. This reward may be difficult to specify, and may also fail to capture the complexity of the desired task. Therefore, it is likely that some materials generated by these methods may be inadequate when it comes to real-world evaluation. For example, materials might be difficult to synthesise, or have undesirable properties such as toxicity which is difficult to eliminate during training. Therefore, we argue SyMDis can be introduced into a material generation workflow, taking advantage of more thorough methods of evaluation to filter out poorly performing candidates. Generative models can be used to learn useful representations from large datasets or large combinatorial spaces, where they can apply cheap computations (e.g., a masking operation with next token prediction, or a cheap reward function), whilst SyMDis can apply more thorough (and possibly more expensive) downstream computations. We propose that such an integration can combine the benefits of both approaches to generate material candidates that are more likely to yield desirable real-world properties, with an interpretable explanation as to why these materials have been selected. This will be considered in future work.% and increase our chances of finding the ``needle(s)" in the haystack. %A high-level overview is shown in Figure \ref{fig:workflow}.

% \begin{figure}[h]
%     \centering
%     \includegraphics[width=0.9\textwidth]{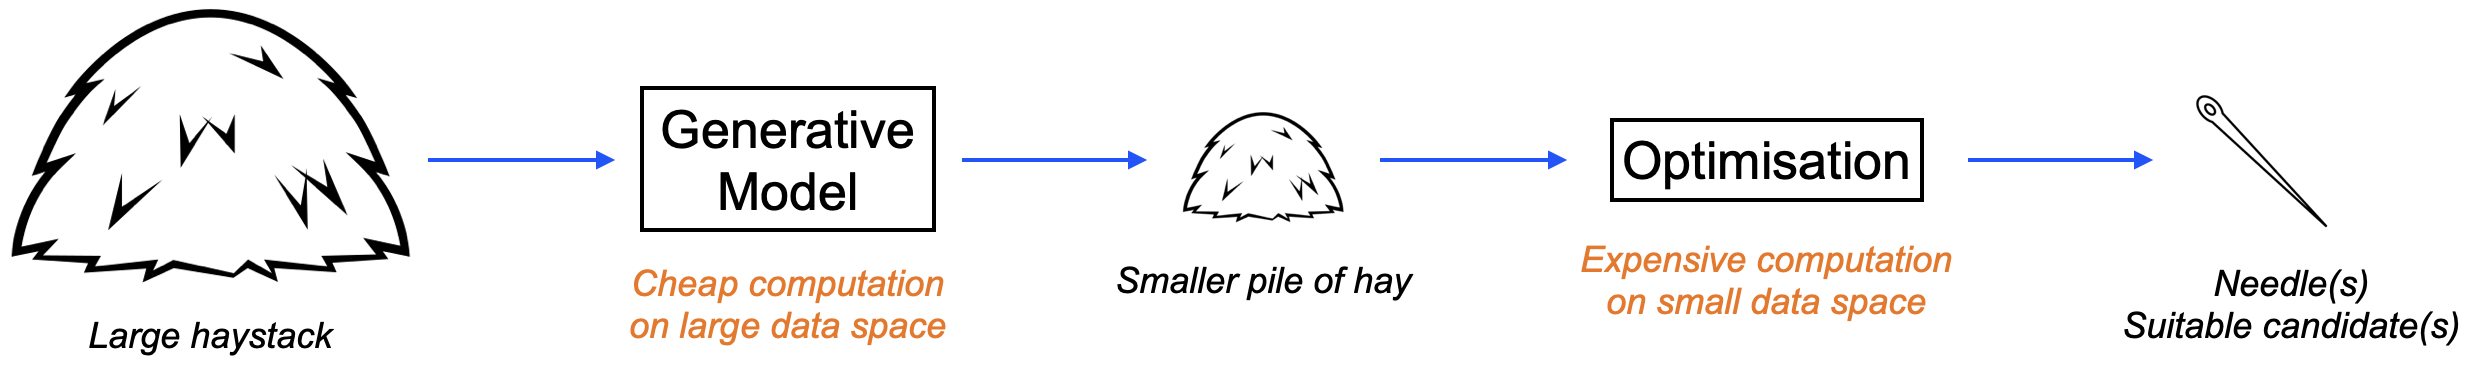}
%     \caption{Proposed workflow integrating SyMDis with generative architectures}
%     \label{fig:workflow}
% \end{figure}

% TODO: also possible to form a loop where we influence the human design of the reward function for a GFlowNet. Maybe this is future work and we leave all of this out?

\textbf{Optimisation of multiple objectives} It would also be interesting to use SyMDis for multi-objective optimisation, such as maximising the working capacity whilst also minimising the cost of production. This could be incorporated by designing a target objective that incorporates multiple metrics (e.g., maximise \textit{target objective} = \textit{working capacity} - \textit{cost}. Another metric to explore would be selectivity, which accounts for how well a MOF can capture only $\mathrm{CO_2}$ given a mixture of gases.

\textbf{Transferability to other domains} The SyMDis method is general and could be applied in other domains. This would be interesting to explore in future work. One point to note is that in more complex tasks, it is unclear whether SyMDis would become stuck in a local optima. This could be mitigated by adding an exploration component (similar to the exploration vs exploitation sampling component in Bayesian Optimisation). In our experiments for CO2 capture, we tried adding a random batch of samples on each iteration (in addition to those selected by the rules), but it didn’t make a difference to the performance. Furthermore, using a logic-based symbolic learner such as FastLAS can help the learned rules generalise and avoid over-fitting to a particular set of examples.
